# Supplementary material for: Ultrarelativistic electron beam polarization in single-shot interaction with an ultraintense laser pulse
Source: arXiv:1812.07229 source file (2018-12-18)
Supplement: Supplementary file 1 [file SM_spin1.pdf]

# Supplemental Materials

## I. THE ELECTROMAGNETIC FIELDS OF THE LASER PULSES

In this work, we employ an elliptically polarized (EP) tightly-focused laser pulse with a Gaussian temporal profile, which propagates along $+z$ direction as a scattering laser beam. The spatial distribution of the electromagnetic fields takes into account up to $\epsilon_0^3$-order of the nonparaxial solution, where $\epsilon_0 = w_0/z_r$, while $w_0$ is the laser focal radius, $z_r = k_0 w_0^2/2$ the Rayleigh length with laser wave vector $k_0 = 2\pi/\lambda_0$, and $\lambda_0$ the laser wavelength. The EP laser pulse can be assumed to be the combination of two orthogonal linearly-polarized (LP) laser pulses, polarizing along $x$ and $y$ directions, respectively, with a $\pi/2$ phase delay, and the expressions of the electromagnetic fields are presented in the following [63, 64]:

$$E_x = E_x^{(1)} + E_x^{(2)}, \quad E_y = E_y^{(1)} + E_y^{(2)}, \quad E_z = E_z^{(1)} + E_z^{(2)},$$
$$B_x = B_x^{(1)} + B_x^{(2)}, \quad B_y = B_y^{(1)} + B_y^{(2)}, \quad B_z = B_z^{(1)} + B_z^{(2)},$$

where,

$$\begin{aligned}
E_x^{(1)} &= -iE^{(1)}\left[1 + \epsilon_0^2\left(f^2\tilde{x}^2 - \frac{f^3\rho^4}{4}\right)\right],\\
E_y^{(1)} &= -iE^{(1)}\epsilon_0^2 f^2\widetilde{xy},\\
E_z^{(1)} &= E^{(1)}\left[\epsilon_0 f\tilde{x} + \epsilon_0^3\tilde{x}\left(-\frac{f^2}{2} + f^3\rho^2 - \frac{f^4\rho^4}{4}\right)\right],\\
B_x^{(1)} &= 0,\\
B_y^{(1)} &= -iE^{(1)}\left[1 + \epsilon_0^2\left(\frac{f^2\rho^2}{2} - \frac{f^3\rho^4}{4}\right)\right],\\
B_z^{(1)} &= E^{(1)}\left[\epsilon_0 f\tilde{y} + \epsilon_0^3\tilde{y}\left(\frac{f^2}{2} + \frac{f^3\rho^2}{2} - \frac{f^4\rho^4}{4}\right)\right];\\
E_x^{(2)} &= -iE^{(2)}\epsilon_0^2 f^2\widetilde{xy},\\
E_y^{(2)} &= -iE^{(2)}\left[1 + \epsilon_0^2\left(f^2\tilde{y}^2 - \frac{f^3\rho^4}{4}\right)\right],\\
E_z^{(2)} &= E^{(2)}\left[\epsilon_0 f\tilde{y} + \epsilon_0^3\tilde{y}\left(-\frac{f^2}{2} + f^3\rho^2 - \frac{f^4\rho^4}{4}\right)\right],\\
B_x^{(2)} &= iE^{(2)}\left[1 + \epsilon_0^2\left(\frac{f^2\rho^2}{2} - \frac{f^3\rho^4}{4}\right)\right],\\
B_y^{(2)} &= 0,\\
B_z^{(2)} &= -E^{(2)}\left[\epsilon_0 f\tilde{x} + \epsilon_0^3\tilde{x}\left(\frac{f^2}{2} + \frac{f^3\rho^2}{2} - \frac{f^4\rho^4}{4}\right)\right];\\
E^{(1)} &= E_0 F_n f e^{-f\rho^2} e^{i(\eta+\psi_{\rm CEP})} e^{-\frac{t^2}{\tau^2}},\\
E^{(2)} &= \epsilon E_0 F_n f e^{-f\rho^2} e^{i(\eta+\pi/2+\psi_{\rm CEP})} e^{-\frac{t^2}{\tau^2}},
\end{aligned} \tag{1}$$

The superscripts $^{(1)}$ and $^{(2)}$ denote the laser pulses linearly-polarized along $x$ and $y$ directions, respectively. $\tau$ is the laser pulse duration, $\epsilon$ the ellipticity, and $E_0$ the amplitude of the laser fields linearly-polarized along $x$ direction with normalization factor $F_n = i$ to keep $\sqrt{(E_x^{(1)})^2 + (E_y^{(1)})^2 + (E_z^{(1)})^2} = E_0$ at the focus, yielding the scaled coordinates

$$\tilde{x} = \frac{x}{w_0}, \quad \tilde{y} = \frac{y}{w_0}, \quad \tilde{z} = \frac{z}{z_r}, \quad \rho^2 = \tilde{x}^2 + \tilde{y}^2, \tag{2}$$

where $f = \frac{i}{\tilde{z}+i}$, $\eta = \omega_0 t - k_0 z$, and $\psi_{\rm CEP}$ is the carrier-envelope phase.

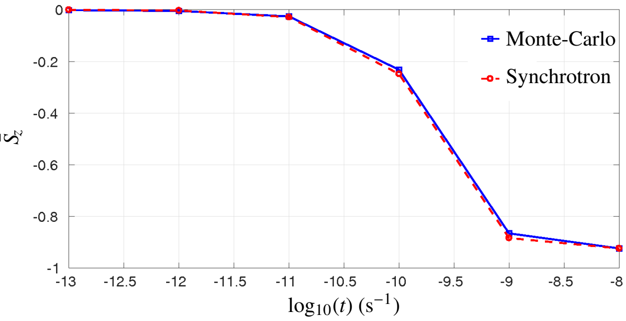


FIG. 1. Simulation of synchrotron radiation. The average spin $\overline{S}_z$ vs the interaction time $t$. The parameters are given in the text.

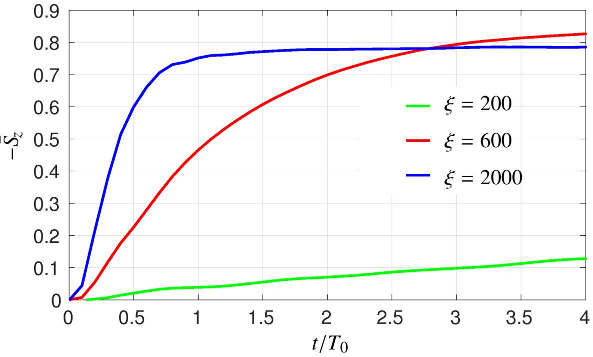


FIG. 2. Simulation of the spin polarization in a rotating electric field. The green, red and blue curves indicate $\xi$ = 200, 600 and 2000, respectively. Other parameters are given in the text.

## II. THE SIMULATION METHOD OF ELECTRON DYNAMICS

The electron dynamics is govern by the classical equations of motion $d\mathbf{p}/dt = -e(\mathbf{E} + \boldsymbol{\beta} \times \mathbf{B})$. Given the smallness of the emission angle $\sim 1/\gamma$ for an ultrarelativistic electron, the photon emission is assumed to be along the electron velocity. The photon emission induces the electron momentum change $\mathbf{p}_f \approx (1 - \hbar\omega_\gamma/c|\mathbf{p}_i|)\mathbf{p}_i$, where $\mathbf{p}_{i,f}$ are the electron momentum before and after the emission, respectively. In this simulation, the interference effects between emissions in adjacent coherent lengths are negligible since the laser fields employed are super-strong, i.e., $\xi \gg 1$. Therefore, the photon emissions happening in each coherent length are independent of each other.

One laser period contains $\xi$ coherence lengths. Here, $\xi \equiv |e|E_0/(m\omega_0 c)$ is the invariant laser field parameter, $E_0$

and $\omega_0$ are the amplitude and frequency of the laser field, respectively, $\gamma$ is the electron Lorentz factor, $c$ the light speed in vacuum, $e$ and $m$ are the electron charge and mass, respectively. And, at each coherence length, the radiation probability is approximately $\alpha$ [46], with the fine structure constant $\alpha$. Thus, in a laser pulse, the emitted photon number $N_{ph} \sim \xi\alpha\tau/T_0$, with the laser period $T_0$.

## III. SIMULATIONS OF SOKOLOV-TERNOV EFFECT

To confirm the accuracy of our Monte-Carlo method, we reproduce the simulations of Sokolov-Ternov effect [17, 18]. In Fig. I, we consider a case of synchrotron radiation. The static magnetic field $B_s$ is along $+z$ direction, and $B_s = \chi B_c/\gamma$, with the critical magnetic field $B_c = \frac{m^2c^3}{e^2\hbar}$ and $\chi = 0.01$. The electron beam is assumed to inject towards $+x$ direction with an initial mean energy $\varepsilon_0 = 1$ GeV. For computing convenience, the electron energy loss is artificially removed, i.e., the parameter $\chi$ is constant. The red-dashed curve is simulated via the well-known method of the electron radiative polarization in storage rings, which is applicable only as $\chi \ll 1$, see Eq. (3.23) in Ref. [20]. Due to the sokolov-Ternov effect, the final polarization rate is approximately 92%. And, our Monte-Carlo method shows a well coincided result, see the blue-solid curve. Note that as the electron energy loss due to the radiation is taken into account, much longer time is required to achieve the high polarization.

Moreover, we also resimulate the spin polarization of an electron beam in a rotating electric field, analogous to the Sokolov-Ternov effect, in Refs. [42, 43]. A particular laser configuration of counter-propagating circularly-polarized plane-waves is considered:

$$E_x = E_0\cos(k_0 z)\cos(\omega_0 t),$$
$$E_y = E_0\cos(k_0 z)\sin(\omega_0 t),$$
$$E_z = 0,$$

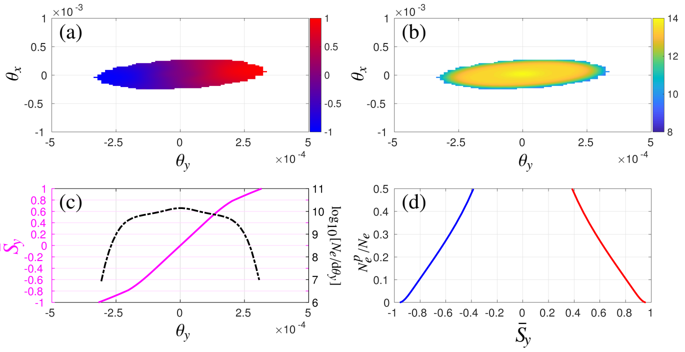


FIG. 3. (a) Transverse distribution of the electron spin component $S_y$ vs the deflection angles $\theta_x = \arctan(p_x/p_z)$ and $\theta_y = \arctan(p_y/p_z)$; (b) Transverse distribution of the electron density $\log_{10}\left(d^2N_e/d\theta_x d\theta_y\right)$ rad$^{-2}$. (c) Average spin $\overline{S}_y$ (magenta solid) and electron distribution $\log_{10}(dN_e/d\theta_y)$ (black dashed) vs $\theta_y$. (d) Ratio of polarized electron number $N_e^p$ to total electron number $N_e$ vs the beam average spin $\overline{S}_y$. The red (right) and blue (left) curves represent the polarization parallel and anti-parallel to the $+y$ axis, respectively. The angular divergence is 0, and other laser and electron beam parameters are the same as in Fig. 2 in the paper.

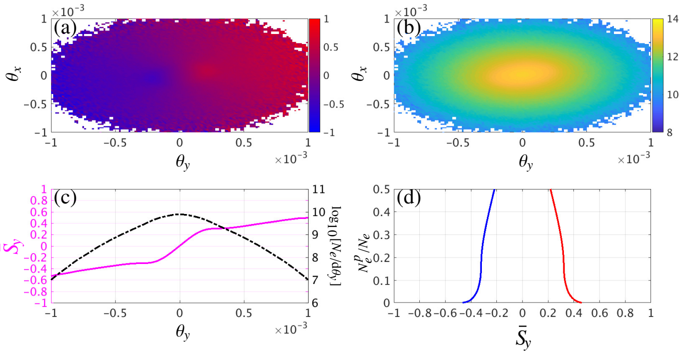


FIG. 4. (a) Transverse distribution of $S_y$ vs $\theta_x$ and $\theta_y$; (b) $\log_{10}\left(d^2N_e/d\theta_x d\theta_y\right)$ rad$^{-2}$. (c) Average spin $\overline{S}_y$ (magenta solid) and electron distribution $\log_{10}(dN_e/d\theta_y)$ (black dashed) vs $\theta_y$. (d) $N_e^p/N_e$ vs $\overline{S}_y$. The red (right) and blue (left) curves represent the polarization parallel and anti-parallel to the $+y$ axis, respectively. The angular divergence is 0.3 mrad, and other laser and electron beam parameters are the same as in Fig. 2 in the paper.

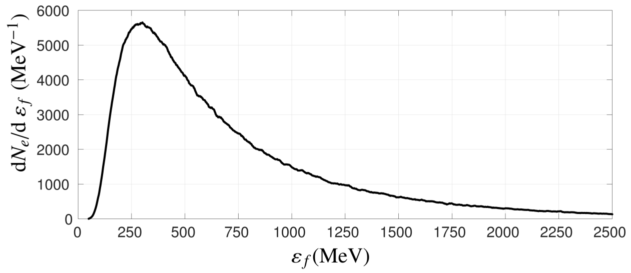


FIG. 5. The electron density distribution with respect to the electron energy after the interaction $\varepsilon_f$. $N_e$ is the electron number. And, the laser and electron beam parameters are the same as in Fig. 2 in the paper.

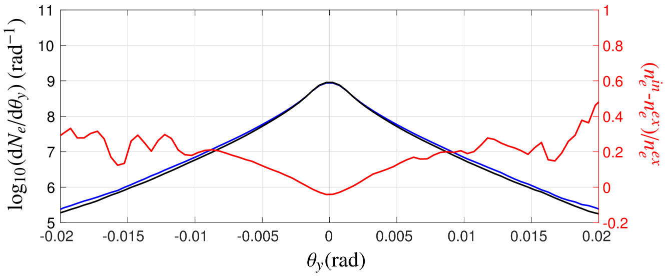


FIG. 6. Spin effects on the electron density distribution. Electron density $n_e = \log_{10}(dN_e/d\theta_y)$ vs $\theta_y$. Blue and black curves includes and excludes the spin effects, respectively. $n_e^{in}$ and $n_e^{ex}$ denote the electron densities in the blue and black curves, respectively.

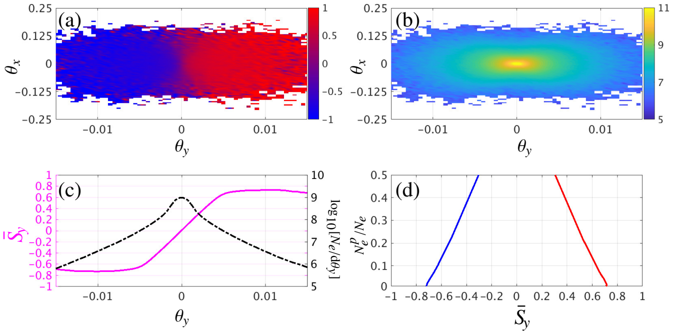


FIG. 7. The role of a large energy spread of the electron beam. (a) and (b): Transverse distributions of electron spin component $S_y$ and density $\log_{10}\left(\mathrm{d}^2N_e/\mathrm{d}\theta_x\mathrm{d}\theta_y\right)$ rad$^{-2}$ with respect to the deflection angles $\theta_x$ and $\theta_y$, respectively. (c) Average spin $\overline{S}_y$ (magenta curve) and electron density $\log_{10}(\mathrm{d}N_e/\mathrm{d}\theta_y)$ (black curve) vs $\theta_y$. (d) $N_e^p/N_e$ vs $\overline{S}_y$. The red and blue curves represent the electrons polarizing parallel and anti-parallel to the $+y$ axis, respectively. The energy spread $\Delta\varepsilon_0/\varepsilon_0 = 0.1$, and other laser and electron beam parameters are the same as in Fig. 2 in the paper.

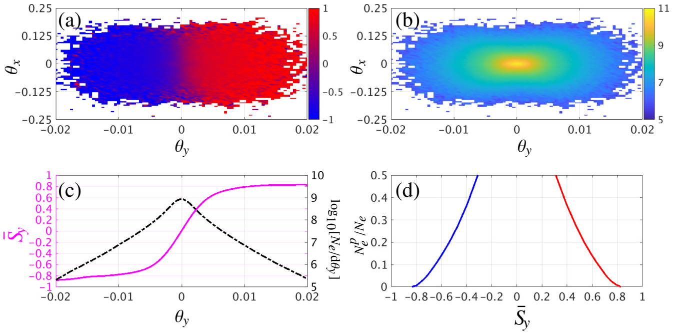


FIG. 8. The role of a large angular spread of the electron beam. (a) and (b): Transverse distributions of electron spin component $S_y$ and density $\log_{10}\left(\mathrm{d}^2N_e/\mathrm{d}\theta_x\mathrm{d}\theta_y\right)$ rad$^{-2}$ with respect to the deflection angles $\theta_x$ and $\theta_y$, respectively. (c) Average spin $\overline{S}_y$ (magenta curve) and electron density $\log_{10}(\mathrm{d}N_e/\mathrm{d}\theta_y)$ (black curve) vs $\theta_y$. (d) $N_e^p/N_e$ vs $\overline{S}_y$. The red and blue curves represent the electrons polarizing parallel and anti-parallel to the $+y$ axis, respectively. The angular divergence of the electron beam is 1 mrad, and other laser and electron beam parameters are the same as in Fig. 2 in the paper.

$$B_x = E_0\sin(k_0z)\cos(\omega_0t),$$
$$B_y = E_0\sin(k_0z)\sin(\omega_0t),$$
$$B_z = 0.$$

As shown in Fig. I, as $\xi$ increases from 200 to 2000, the polarization speed increases dramatically. Our method represents uniform results compared with those in [42, 43].

More interesting point is that our method is applicable for arbitrary electromagnetic fields.

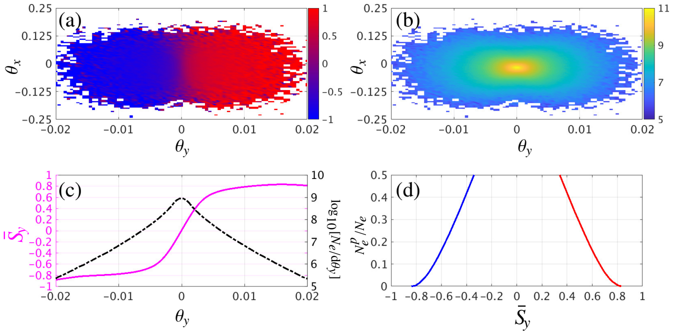


FIG. 9. The role of the laser and electron beam alignment. (a) and (b): Transverse distributions of electron spin component $S_y$ and density $\log_{10}\left(\mathrm{d}^2N_e/\mathrm{d}\theta_x\mathrm{d}\theta_y\right)$ rad$^{-2}$ with respect to the deflection angles $\theta_x$ and $\theta_y$, respectively. (c) Average spin $\overline{S}_y$ (magenta curve) and electron density $\log_{10}(\mathrm{d}N_e/\mathrm{d}\theta_y)$ (black curve) vs $\theta_y$. (d) $N_e^p/N_e$ vs $\overline{S}_y$. The red and blue curves represent the electrons polarizing parallel and anti-parallel to the $+y$ axis, respectively. The colliding polar angle $\theta_e = 179°$, and other laser and electron beam parameters are the same as in Fig. 2 in the paper.

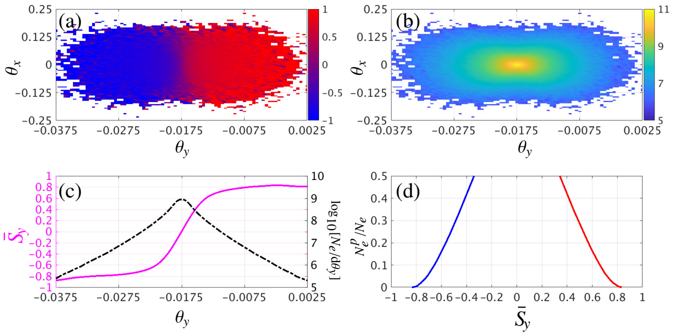


FIG. 10. The role of the laser and electron beam alignment. (a) and (b): Transverse distributions of electron spin component $S_y$ and density $\log_{10}\left(\mathrm{d}^2N_e/\mathrm{d}\theta_x\mathrm{d}\theta_y\right)$ rad$^{-2}$ with respect to the deflection angles $\theta_x$ and $\theta_y$, respectively. (c) Average spin $\overline{S}_y$ (magenta curve) and electron density $\log_{10}(\mathrm{d}N_e/\mathrm{d}\theta_y)$ (black curve) vs $\theta_y$. (d) $N_e^p/N_e$ vs $\overline{S}_y$. The red and blue curves represent the electrons polarizing parallel and anti-parallel to the $+y$ axis, respectively. The colliding polar angle $\theta_e = 179°$ and azimuthal angle $\phi_e = 90°$, and other laser and electron beam parameters are the same as in Fig. 2 in the paper.

## IV. MODIFIED LANDAU-LIFSHITZ EQUATION ACCOUNTING FOR RADIATIVE SPIN EFFECTS

Generally, the Landau-Lifshitz (LL) equation [70] describes electron dynamics under the action of radiation reaction (RR) in the classical regime $\chi \ll 1$. In the case of $\chi \sim 1$, the classical LL model overestimates the RR force, which is remedied phenomenologically in the modified LL model [46, 66].

The RR is considered as the effect of the electromagnetic fields emitted by an electron on the motion of itself classically. The dynamics of an electron is discribed by the LL equation [70]

$$m\frac{\mathrm{d}v^\mu}{\mathrm{d}\tilde{\tau}} = eF^{\mu j}v_j + f^\mu, \tag{3}$$

where

$$f^{\mu} = \frac{2e^3}{3mc^2}(\partial_\alpha F^{\mu\nu} v_\nu v^\alpha) + \frac{2e^4}{3m^2c^4}(F^{\mu\nu} F_{\nu\alpha} v^\alpha + (F^{\nu\beta} v_\beta F_{\nu\alpha} v^\alpha) v^\mu), \tag{4}$$

$v = (\gamma, \gamma \mathbf{v}/c)$ is four-velocity of the electron, $\tilde{\tau}$ the proper time,

$$\frac{\mathrm{d}}{\mathrm{d}\tilde{\tau}} = (k \cdot p)\frac{\mathrm{d}}{\mathrm{d}\eta}, \quad \eta = (k \cdot \tilde{r}), \tag{5}$$

$F_{\mu\nu}$ is the field tensor, $p$, $k$, and $\tilde{r}$ are 4-vectors of the electron momentum before radiation, laser wave-vector, and coordinate, respectively. The three-dimention equation is

$$\begin{aligned}\mathbf{F}_C = \frac{2e^3}{3mc^3}\Bigg(\gamma\left(\left(\frac{\partial}{\partial t} + \frac{\mathbf{p}}{\gamma m}\cdot\nabla\right)\mathbf{E} + \frac{\mathbf{p}}{\gamma mc}\times\left(\frac{\partial}{\partial t} + \frac{\mathbf{p}}{\gamma m}\cdot\nabla\right)\mathbf{B}\right)\\ + \frac{e}{mc}\left(\mathbf{E}\times\mathbf{B} + \frac{1}{\gamma mc}\mathbf{B}\times(\mathbf{B}\times\mathbf{p}) + \frac{1}{\gamma mc}\mathbf{E}(\mathbf{p}\cdot\mathbf{E})\right)\\ - \frac{e\gamma}{m^2c^2}\mathbf{p}\left(\left(\mathbf{E} + \frac{\mathbf{p}}{\gamma mc}\times\mathbf{B}\right)^2 - \frac{1}{\gamma^2 m^2 c^2}(\mathbf{E}\cdot\mathbf{p})^2\right)\Bigg),\end{aligned} \tag{6}$$

where, $\mathbf{E}$ and $\mathbf{B}$ are the electric and magnetic fields, respectively, and, $\mathbf{p}$ is the electron momentum.

We treat the electron dynamics in the external field semi-classically including the quantum-recoil and spin effects. The equation used to calculate the electron dynamics is the modified-LL equation with the classical RR force in the LL equation replaced by the quantum RR force:

$$\mathbf{F}_{QED} = \frac{I_{QED}}{I_C}\mathbf{F}_C, \tag{7}$$

where,

$$I_{QED} = mc^2 \int c\,(k \cdot k')\,\frac{\mathrm{d}W_{fi}}{\mathrm{d}u\mathrm{d}\eta}\mathrm{d}u, \tag{8}$$

$$I_C = \frac{2e^4 E'^2}{3m^2c^3}, \tag{9}$$

and $\frac{\mathrm{d}W_{fi}}{\mathrm{d}u\mathrm{d}\eta}$ is the spin-dependent radiation probability in Eq. (2) of the paper. Here, $E'$ is the electric fields in the electron frame. $k'$ and $p_i$ are the four-vector of the wave vector of the emitted photon and the momentum of the electron before the radiation, respectively.

We resimulate the results in Fig. 2 in the paper by a semi-classical model: the electron motion is governed by Modified LL Model including the quantum-recoil and spin effects; the electron spin precession is governed by the Thomas-Bargmann-Michel-Telegdi equation, but the spin flips are artificially removed. The results are shown in Figs. 3 and 4 with an angular divergence of 0 and 0.3 mrad, respectively, which show qualitatively uniform results and confirm the rationality of our Monte-Carlo method in the paper. Compared with Fig. 2 in the paper, the splitting angles in this semi-classical model are much smaller, since the stochasticity effects of photon emission are neglected artificially. And, as the angular divergence increases from 0 to 0.3 mrad, even though the splitting angle increases as well, more polarized electrons near $\theta_y = 0$ overlap, and consequently, the polarization rate declines.

## V. ELECTRON ENERGY DENSITY AFTER THE INTERACTION AND SPIN EFFECTS ON THE ELECTRON DENSITY DISTRIBUTION

The electron density distribution with respect to the electron energy after the interaction is shown in Fig. 5. The peak energy is approximately 300 MeV ($\gamma \approx 587$), and consequently, the angular divergence of the electrons is roughly 1.7 mrad, which is much smaller than the splitting angle in Fig. 2 in the paper.

The spin effects on the electron density distribution are shown in Fig. 6. The relative difference is shown as $(n_e^{in}$-$n_e^{ex})/n_e^{ex}$, see the red curve. As $|\theta_y|$ increases, the relative difference ascends as well up to roughly 40%.

## VI. IMPACTS OF LASER AND ELECTRON BEAM PARAMETERS ON THE POLARIZATION

For the experimental convenience, we investigate the impacts of the laser and elecron beam parameters on the polarization. In Figs. 7-10, the cases of larger energy spread $\Delta\varepsilon_0/\varepsilon_0 = 0.1$, larger angular divergence of 1 mrad, colliding polar angle of the electron beam $\theta_e = 179°$, and colliding azimuthal angle $\phi_e = 90°$ are calculated, respectively. Other parameters are the same as in Fig. 2 in the paper. As those parameters vary in an experiment, the signatures of the electron beam spin-polarizing and splitting quantitatively keep stable and are uniform with those in Fig. 2 in the paper.
